# Supplementary material for: Theory and computation of Hall scattering factor in graphene
Source: arXiv:2111.10774 source file (2021-11-21)
Supplement: Supplementary file 1 [file Supplementary.pdf]

# Supplementary Information to "Theory and computation of Hall scattering factor in graphene"


Francesco Macheda* and Nicola Bonini†

*Department of Physics, King's College London, Strand, London WC2R 2LS, United Kingdom*

Samuel Ponce‡

*Department of Materials, University of Oxford, Parks Road, Oxford OX1 3PH, United Kingdom and*
*Theory and Simulation of Materials (THEOS), École Polytechnique Fédérale de Lausanne, CH-1015 Lausanne, Switzerland*

Feliciano Giustino§

*Oden Institute for Computational Engineering and Sciences,*
*The University of Texas at Austin, Austin, Texas 78712, USA and*
*Department of Physics, The University of Texas at Austin, Austin, Texas 78712, USA*



* francesco.macheda@kcl.ac.uk
† nicola.bonini@kcl.ac.uk
‡ samuel.ponce@epfl.ch
§ fgiustino@oden.utexas.edu

## I. THEORY AND GENERAL COMPUTATIONAL STRATEGIES

The Boltzmann equation for electrons may be written as (using $e = \hbar = 1$ and the same notation as [1, 2]):

$$\left[1 - \tau^{(0)}_{n\mathbf{k}}(\mathbf{v}_{n\mathbf{k}} \wedge \mathbf{B}) \cdot \frac{\partial}{\partial \mathbf{k}}\right] \partial_{E_\beta} f_{n\mathbf{k}} = \frac{\partial f^0_{n\mathbf{k}}}{\partial \epsilon_{n\mathbf{k}}} v_{n\mathbf{k},\beta} \tau^{(0)}_{n\mathbf{k}} + 2\pi \tau^{(0)}_{n\mathbf{k}} \sum_{m\nu} \int \frac{d\mathbf{q}}{\Omega_{BZ}} |g_{mn\nu}(\mathbf{k},\mathbf{q})|^2 \times$$
$$\left[(1 + n_{\mathbf{q}\nu} - f^0_{n\mathbf{k}})\delta(\epsilon_{n\mathbf{k}} - \epsilon_{m\mathbf{k}+\mathbf{q}} + \omega_{\mathbf{q}\nu}) + (n_{\mathbf{q}\nu} + f^0_{n\mathbf{k}})\delta(\epsilon_{n\mathbf{k}} - \epsilon_{m\mathbf{k}+\mathbf{q}} - \omega_{\mathbf{q}\nu})\right]. \quad (1)$$

where $\mathbf{B}$ is the magnetic field, the set $\{n\mathbf{k}\}$ is associated to a certain electronic energy band $n$ of a certain quasi-momentum $\mathbf{k}$, $f_{n\mathbf{k}}$ is the out of equilibrium electronic population, $f^0_{n\mathbf{k}}$ is the equilibrium Fermi-Dirac electronic population, $\mathbf{v}_{n\mathbf{k}}$ is the electronic band velocity, $\epsilon_{n\mathbf{k}}$ is the band energy, $g_{mn\nu}(\mathbf{k},\mathbf{q})$ is the coupling between electron and phonons [3], the set $\{\mathbf{q}\nu\}$ is associated to a certain phonon energy branch $\nu$ of a certain momentum $\mathbf{q}$, $n_{\mathbf{q}\nu}$ is the phonon population (always considered at equilibrium in this work), $\omega_{\mathbf{q}\nu}$ is the phonon energy , $\Omega_{BZ}$ is the Brillouin Zone volume (or area) and $\tau^{(0)}_{n\mathbf{k}}$is defined as:

$$\frac{1}{\tau^{(0)}_{n\mathbf{k}}} = 2\pi \sum_{m\nu} \int \frac{d\mathbf{q}}{\Omega_{BZ}} |g_{mn\nu}(\mathbf{k},\mathbf{q})|^2 \times \left[(1 + n_{\mathbf{q}\nu} - f^0_{m\mathbf{k}+\mathbf{q}})\delta(\epsilon_{n\mathbf{k}} - \epsilon_{m\mathbf{k}+\mathbf{q}} - \omega_{\mathbf{q}\nu}) + (n_{\mathbf{q}\nu} + f^0_{m\mathbf{k}+\mathbf{q}})\delta(\epsilon_{n\mathbf{k}} - \epsilon_{m\mathbf{k}+\mathbf{q}} + \omega_{\mathbf{q}\nu})\right]. \quad (2)$$

Its exact solution (with or without magnetic field) can be achieved via iterative or CG schemes [1, 4, 5]; this usually requires very fine grids of equally dimensioned $\mathbf{k}/\mathbf{q}$-point grids (a different grid for the $\mathbf{q}$-points may be used to evaluate for example $\tau^{(0)}_{n\mathbf{k}}$ but, if different grids are used in the full solution, spurious non-physical oscillations appear in the out of equilibrium population $f_{n\mathbf{k}}$).

The quantities $f^0_{n\mathbf{k}}, \epsilon_{n\mathbf{k}}, \mathbf{v}_{n\mathbf{k}}, n_{\mathbf{q}\nu}, \omega_{\mathbf{q}\nu}, \tau^{(0)}_{n\mathbf{k}}$ can be calculated just on the Irreducible Wedge (IW) of the Brillouin Zone (BZ) and then associated to the $\mathbf{k}/\mathbf{q}$-points of the full grid through the appropriated symmetry operations that belong to the star of a given $\mathbf{k}$. $\epsilon_{n\mathbf{k}}, \mathbf{v}_{n\mathbf{k}}, \omega_{\mathbf{q}\nu}$ can be obtained via an efficient Wannier interpolation scheme [6, 7].

As regards $g_{mn\nu}(\mathbf{k},\mathbf{q})$, it can be interpolated on fine $\mathbf{k}/\mathbf{q}$-point grids via Wannier interpolation [6] choosing $\mathbf{k} \in IW$ and $\mathbf{q} \in BZ$; the value on the whole grid can then be obtained by using the relation [4]:

$$|g_{mn\nu}(\mathbf{k},\mathbf{q})|^2 = |g_{mn\nu}(S\mathbf{k}, S\mathbf{q})|^2 \quad (3)$$

where $S$ is one of the symmetry operations associated with the star of $\mathbf{k}$. The previous relation hold for non-degenerate states, while for degenerate bands/phonons we just know that:

$$\sum_{mn\nu} |g_{mn\nu}(\mathbf{k},\mathbf{q})|^2 = \sum_{mn\nu} |g_{mn\nu}(S\mathbf{k}, S\mathbf{q})|^2 \quad (4)$$

because of the gauge freedom within degenerate subspaces. A proper modification of the Boltzmann equation where $\mathbf{v}_{n\mathbf{k}}$ is substituted by the matrix elements $\mathbf{v}_{n\mathbf{k},m\mathbf{k}'}$ (defined as in [7]) and $f_{n\mathbf{k}}$ by $f_{n\mathbf{k},m\mathbf{k}}$ should be implemented to make the equation properly gauge invariant in degenerate subspaces (see for example [8] for an homogeneous system). Nonetheless, the set of points with degeneracy in a crystal is usually of null measure and therefore for practical reasons this is not done. We also remind that the gauge freedom for the phonon modes does not affect the final results because the phonon branches always appear as summed over in the Boltzmann equation. Therefore, practically for $|g|^2$ we treat the degeneracy points as if they were non-degenerate and then check that our grids are big enough to leave the results unaffected by the gauge choice; for $\mathbf{v}$, we adopt the gauge such that at each point the velocity matrix is diagonal and respects the lattice symmetry, so that transport quantities are recovered in the correct symmetrical form. In the present work, the degeneracy point is just the Dirac cone center so the result is almost immediately gauge invariant. In passing by, we also mention that the property of Eq. 3 for symmetric operations belonging to the small group of $\mathbf{k}$ becomes:

$$|g_{mn\nu}(\mathbf{k},\mathbf{q})|^2 = |g_{mn\nu}(S\mathbf{k}, S\mathbf{q})|^2 = |g_{mn\nu}(\mathbf{k}, S\mathbf{q})|^2 \quad (5)$$

so that this property usually needs to be enforced numerically.

In principle, Eq. 1 has to be solved for each $\mathbf{k}$-point and for each band $n$. In practice, the transport quantities depends just on a small region of energies around the Fermi level. In particular, we are interested in the electrical conductivity tensor:

$$\sigma_{\alpha\beta}(\mathbf{B}) = -\frac{2}{\Omega N_{\mathbf{k}}} \sum_{n\mathbf{k}} \frac{\partial f^0_{n\mathbf{k}}}{\partial \epsilon_{n\mathbf{k}}} v_{n\mathbf{k},\alpha} \partial_{E_\beta} f_{n\mathbf{k}} \quad (6)$$

where $\Omega$ is the volume (or area) of the primitive cell and the factor 2 accounts for spin degeneration (which we consider as never lifted in this work). As from Eq. 6, it is clear that $\frac{\partial f^0_{n\mathbf{k}}}{\partial \epsilon_{n\mathbf{k}}}$ saves the contributions of the out of equilibrium populations just around the Fermi energy. Indeed, also the out of equilibrium population themselves are substantially different from the in equilibrium ones just around the Fermi energy, because the known term of Eq. 1 contains $\frac{\partial f^0_{n\mathbf{k}}}{\partial \epsilon_{n\mathbf{k}}}$. This consideration can be used to speed up the calculation sensibly by just considering the $\mathbf{k}/\mathbf{k}+\mathbf{q}$-points that generate energies that are inside a certain Fermi surface thickness.

In order to approximate the energy conserving Dirac delta function (as for example the ones appearing in Eq. 2) we adopt two different strategies. The first strategy is to use a normal distribution with a variance which is independent of the argument of the delta. The second strategy is to adopt an "adaptive" variance which is a function of $\epsilon_{n\mathbf{k}} - \epsilon_{m\mathbf{k}'}$; this second way of proceeding is implemented only when computing the contribution to the transport quantities given by the set of $\mathbf{k}$-points in the neighbourhood of the Dirac cone center and it is of particular relevance when studying the linear behaviour of the inverse scattering time (see next sections). In this region, a fixed variance approach performs badly because the $\mathbf{k}$-point sampling obtained via uniform grids is much less dense than in other regions. Finally, we mention that the approximation of the Dirac delta via sharp but finite Gaussians in principle breaks the detailed balance relation. In our calculations we check that this does not affect the final result (see next sections).

| $n$ $(cm^{-2})$ | $\mathbf{k}/\mathbf{q}$-points grids | window $(meV)$ | $\sigma$ $(meV)$ |
|---|---|---|---|
| $5 \times 10^{11} - 9 \times 10^{11}$ | $1404 \times 1404 \times 1$ | 500 | 5 |
| $1 \times 10^{12} - 4 \times 10^{12}$ | $1080 \times 1080 \times 1$ | 500 | 5 |
| $5 \times 10^{12} - 1 \times 10^{13}$ | $1080 \times 1080 \times 1$ | 700 | 5 |

TABLE I. Converged parameters for transport properties

## II. COMPUTATIONAL DETAILS

Our procedure for the calculation of the transport quantities in crystals consists in various steps, as explained in Ref [2, 4, 5]:

1. Self-Consistent-Field (SCF) calculation of the ground state density of the system by means of standard ab-initio DFT techniques [9];
2. Non-Self-Consistent-Field (NSCF) calculation of the wavefunctions $\Psi_{\mathbf{k}n}$ and band structure of the system using the SCF ground state density;
3. Density Functional Perturbation Theory (DFPT) [10] calculation of the phonon spectrum of the system and variation of the electronic Khon-Sham potential $\partial_{\mathbf{q}\nu} V$ with respect to a phonon mode $(\mathbf{q}, \nu)$;
4. Calculation of the Electron Phonon Coupling (EPC) using DFPT $\partial_{\mathbf{q}\nu} V$ and NSCF $\Psi_{\mathbf{k}n}$;
5. Wannier-scheme interpolation [11] of the band structure energies, band velocities, phonon energies and EPC elements on very fine grids;
6. Calculation of the transport properties.

For the first 4 steps we have used the Quantum Espresso (QE) code [12] and for the last 2 we have used a pre-release version of the EPW code [13, 14]. For the SCF calculation, we have used a non-relativistic Norm-Conserving (NC) pseudopotential compatible with the LDA-PZ exchange-correlation functional [15, 16], a plane wave cutoff energy of $100 Ry$ and a $\mathbf{k}$-point grid of dimensions $96 \times 96 \times 1$ to accurately describe the ground state of graphene. The primitive cell is described via the lattice vectors $\mathbf{v}_1 = a(1, 0, 0)$, $\mathbf{v}_2 = a(-1/2, \sqrt{(}3)/2, 0)$, $\mathbf{v}_3 = a(0, 0, c/a)$ where $a = 4.60$ $Bohr$ and $c = 5.0$ ( even though the stability of the values of the EPC matrix elements and of the transport coefficients has been checked against increase of the $c$ parameter up to 10.0). For the NSCF calculation, we have used the same parameters but we have used a $\mathbf{k}$-point grid of dimensions $24 \times 24 \times 1$ (we will show in the next section that this is sufficient). The doping has been simulated within the rigid band approximation; such approximation is not appropriate for flexural phonons and for the "deformation potential" terms of the EPC, but those terms do not contribute relevantly to transport in graphene [17]. For the phonon calculations, we have used a $\mathbf{q}$-point grid of dimensions $24 \times 24 \times 1$ and a tight threshold for convergence of the DFPT calculation (using a self-consistent threshold of $10^{-20}$ for the solution of the Sternheimer linear equation). The EPC has been calculated on the NSCF $\mathbf{k}$ and on the DFPT $\mathbf{q}$-point grids and then has been interpolated, together with the other one particle quantities, on very fine grids via Wannier interpolation. The Wannier interpolation has been done using 5 functions, and the Maximally Localized Wannier functions have spread ranging from $0.6098 \mathring{A}^2$ to $2.7183 \mathring{A}^2$. Finally, we report in table I the converged values for the fine grids, energy window from the Dirac cone and Gaussian smearing that has been used in the calculations of the transport calculations with EPW. All the convergence pictures are given in the next section.

## III. CONVERGENCE OF WANNIER INTERPOLATION AND COMPARISON WITH MODELS

In this section we study the convergence of the interpolation of the ab-initio EPC matrix elements and compare the results with pre-existing models of the interaction. We put ourself near the Dirac cone, at a $\mathbf{k}$-point with cartesian coordinates $\mathbf{k_1} = (0.3437500, 0.5953925, 0)$ (in units of $\frac{2\pi}{a}$, this is a point that belongs to the $48 \times 48 \times 1$ SCF grid and that is on the line that connects the $K$ and $\Gamma$ points) and consider $\mathbf{q}$-points of the form $\mathbf{q} = \lambda \mathbf{k_1}$ with very small $\lambda$, so that we can say that the $\mathbf{q}$ runs on the $\Gamma - K$ line. We compute the ab-initio EPC $\langle n = 4, 5; \mathbf{k_1} + \mathbf{q} | \partial_{\mathbf{q}\nu} V | m = 4, 5; \mathbf{k_1} \rangle$ (4 is the index for the band below the Dirac cone, 5 is the index for the band above) and compare it with its Wannier interpolation obtained for different NSCF and DFPT grids in Panel 1. Since on the $\Gamma - K$ line is a special line we have some symmetry constraints on the EPC elements (as explained in Ref [18]), so that some elements need to be 0 on whole sectors of the line. Such elements provide a very clear indicator for the convergence of the interpolation: from Panel 1 we see that a NSCF $\mathbf{k}$-point grid of $24 \times 24 \times 1$ and a DPT $\mathbf{q}$-point grid of $24 \times 24 \times 1$ catch very well the behaviour of the ab-initio EPC. We also mention that we tested the ab-initio results under change of SCF grid (up to $144 \times 144 \times 1$) and of Gaussian smearing during the SCF cycle, finding no appreciable differences. In passing by, we notice that not all matrix elements (both ab-initio and interpolated) go to 0 when $|\mathbf{q}| \to 0$, in opposition of what is said in Ref [18]; the reason for this is that the Hellmann-Feynman applied to $\Gamma$ acoustic phonons (which are free of non-analyticity in graphene) when $m = n$ reads:

$$\langle \mathbf{k} + \mathbf{q} n | \frac{\partial V^{TA/LA}}{\partial \mathbf{q}} | \mathbf{k} n \rangle |_{\mathbf{q}=0} = \frac{\partial \epsilon_{n\mathbf{k}}}{\partial \mathbf{q}} |_{\mathbf{q}=0} = 0 \quad (7)$$

but this relation does not evaluate to 0 when $n \neq m$ because instead of the Helmann-Feynmann theorem we have the Epstein formula [19]. Moreover also the hole-electron symmetry for the modulus of the EPC matrix elements, which is usually assumed for graphene EPC (see for example Ref [20, 21]), is broken in an ab-initio calculation because the response function in the DFPT calculation depends on the ground state density, which in turn depends only on the occupied states. A part from the above mentioned discrepancies, if we compare the ab-initio result and the Wannier interpolation with models (such as the one in Ref [21]), we find an overall good agreement for the angular dependency of the EPC for the acoustic modes, whereas for the optical phonon the behaviour is oversimplified in such models.

## IV. CONVERGENCE OF TRANSPORT QUANTITIES

In this section we present the convergence of transport quantities with respect to computational parameters. Referring to Panel 2 (a), we first notice the expected (for a 2D material) quadratic scaling of the active **q**-points $N_{\mathbf{q}}^{act.}$ involved in the transport coefficient calculations inside the active energy window; the time of the calculation increases with the **k**/**q**-point grids as $t \propto N_{\mathbf{k}}^{irr.} \times N_{\mathbf{q}}^{act.}$ where $N_{\mathbf{k}}^{irr.}$ is the number of irreducible points for a given grid (see the section above for the use of symmetries). In the same figure we also show the convergence of (b) Fermi energy, (c) drift mobility and (d) Hall coefficient tensor components against the size of the **k**/**q**-point grids, while keeping a fixed smearing of $5meV$ for a carrier density of $10^{12}cm^{-2}$ and an active energy window extending $500meV$ below and above the Dirac cone center. The Fermi level at a given temperature converges to a precision of $10^{-3}eV$ already at grids of dimensions $1080 \times 1080 \times 1$, whereas the difference between Fermi levels at $600K$ and $300K$ (not shown here) converges to a precision of $3 \times 10^{-4}eV$ at the same grid (the center of the Dirac cone is at an energy of $-1.3009eV$). Regarding the convergence of the mobility, we have two different trends for $300K$ and $600K$ that show the difficulty of converging the result at lower temperatures, where in general a smaller region around the Fermi level contributes to transport. At the lowest temperature investigated in this work ($300K$) we have a change of the mobility of $240\frac{cm^2}{Vs}$ (0.1%) at grids of dimensions $1080 \times 1080 \times 1$. As regards the Hall factor, since graphene is not a cubic semiconductor, the cartesian derivatives of the out of equilibrium populations cannot be done when using a uniform **k**-point grid; in this case, we take derivatives along crystal direction and then rotate the resulting gradient to transform it into cartesian coordinates. This operation is justified when the distance between the point tends to 0; the symmetries of the physical quantities are thus recovered in such limit. We can notice that at grids of dimensions $1080 \times 1080 \times 1$ the Hall factor $r^{xy}$ is converged up to $3 \times 10^{-2}$ and $5 \times 10^{-3}$ for $300K$ and $600K$ respectively; the sum $r^{xy} + r^{yx}$, which should be 0 when the physical symmetries are recovered, is in this case $5 \times 10^{-3}$ and $5 \times 10^{-4}$ respectively. In Panel 2 we also show the convergence of the (a) mobility and (b) Hall factor when changing smearing at fixed **k**/**q**-point grids of dimensions $1080 \times 1080 \times 1$ for a density of $10^{12}cm^{-2}$. In this case, we notice that within in the range $2meV \div 20meV$ the transport quantities are quite stable.

Other convergence tests, that we do not report, have been done for different carrier densities. The final converged parameters used in this work are reported in Table I.

## V. MOBILITY, SERTA VS FULL SOLUTION AND CONVERGENCE OF ITERATIONS

Since the Hall scattering factor is a ratio of two components of the conductivity tensor, we start analyzing the drift mobility of a doped graphene sample to compare our calculation with the present literature. Experimental values for the intrinsic mobility of graphene at room temperature show very high values, up to $\sim 200\ 000\ \frac{cm^2}{Vs}$ [22–24]. The values are much higher than traditional semiconductors such as silicon, germanium or gallium-arsenide. Theoretical investigations of the mobility for graphene, done both via models or ab-initio investigations [25–28], also predicts remarkably high values. In this work, we studied both the electron and the hole mobility. Since the difference between the two is quantitatively very small (hole mobility is higher of about 7% at room temperature), we will concentrate just on the hole mobility. The behaviour of the hole mobility as a function of the carrier density is shown in Panel 3 (a). For low doping concentrations, the behaviour of the mobility is roughly $\mu \propto n^{-0.85}$, in good agreement with previous predictions; at higher densities the curve doesn't follow a specific power law and, since in this case the Fermi level falls distant for the center of the Dirac cone, it is impossible to use model to predict the values or the behaviours of the mobility. The temperature behaviour of the hole mobility for different doping concentrations is shown in Panel 3 (b). We have a monotonic descrease of the mobility with increasing temperature, as it qualitatively happens also for traditional semiconductors; for low doping concentrations and around room temperature, we roughly have $\mu \propto T^{-2.2}$. The value obtained for a carrier density of $10^{12}cm^{-2}$ at room temperature is of $\sim 140\ 000\frac{cm^2}{Vs}$, in very good agreement with previous ab-initio calculations and experimental results. In Panel 3 (c) we also show that, upon removal of the scaterring between electrons and phonons with frequencies higher that $60meV$ at a carrier density of $10^{12}cm^{-2}$, the slope of the curve changes from $\mu \propto T^{-2.2}$ to $\mu \propto T^{-0.85}$. This is in good agreement with what is predicted by models in absence of optical phonons [21]. We also checked that the imposition of the quasielastic scattering condition (neglection of phonon frequencies inside the energy-conserving Dirac deltas) still leads to the same temperature power $\mu \propto T^{-0.85}$. We conclude that optical phonons at temperatures near room temperature are important in graphene in order to correctly catch the temperature behaviour of the mobility; a crucial observation though is that optical phonons become less and less important for the value of the mobility as the temperature decreases, and already at 300K the acoustic scattering alone gives a mobility only 30% higher than the value with full interactions. As explained in the main text, the determination of the Hall factor instead includes the optical phonon scattering as a fundamental ingredient even at room temperature.

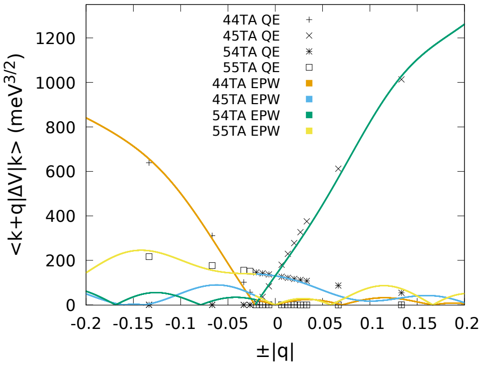


FIG. 1. TA mode, NSCF $24 \times 24 \times 1$ and DFPT $12 \times 12 \times 1$

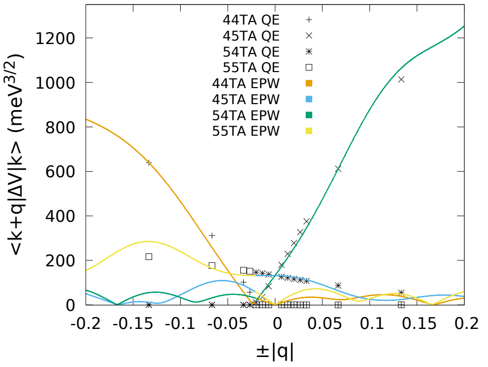


FIG. 2. TA mode, NSCF $48 \times 48 \times 1$ and DFPT $12 \times 12 \times 1$

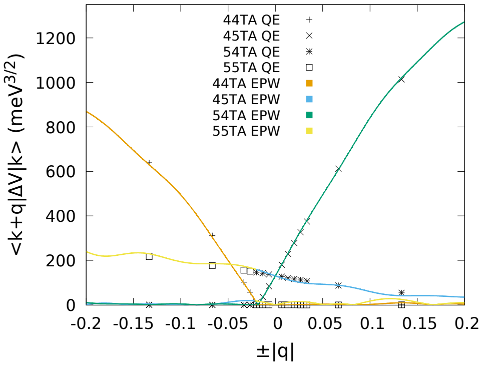


FIG. 3. TA mode, NSCF $24 \times 24 \times 1$ and DFPT $24 \times 24 \times 1$

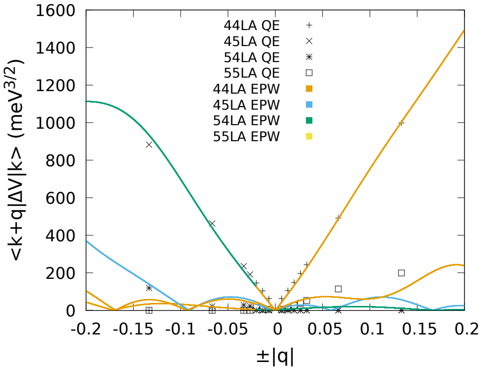


FIG. 4. LA mode, NSCF $24 \times 24 \times 1$ and DFPT $12 \times 12 \times 1$

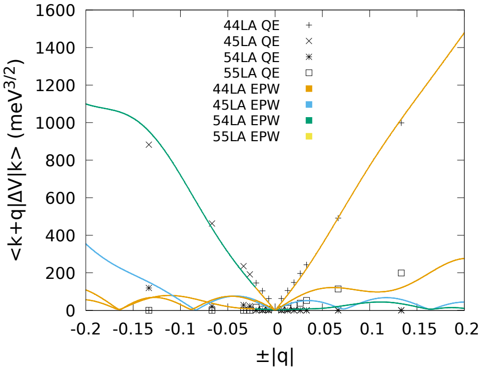


FIG. 5. LA mode, NSCF $48 \times 48 \times 1$ and DFPT $12 \times 12 \times 1$

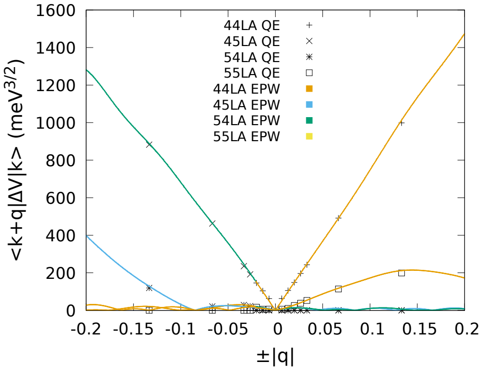


FIG. 6. LA mode, NSCF $24 \times 24 \times 1$ and DFPT $24 \times 24 \times 1$

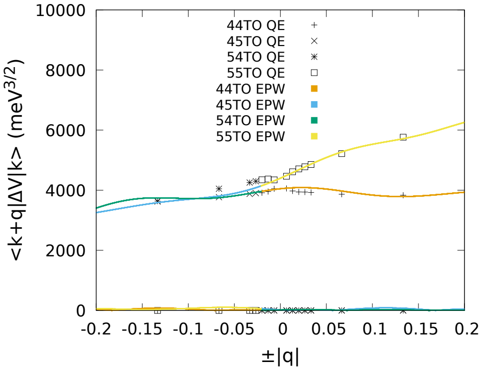


FIG. 7. TO mode, NSCF $24 \times 24 \times 1$ and DFPT $12 \times 12 \times 1$

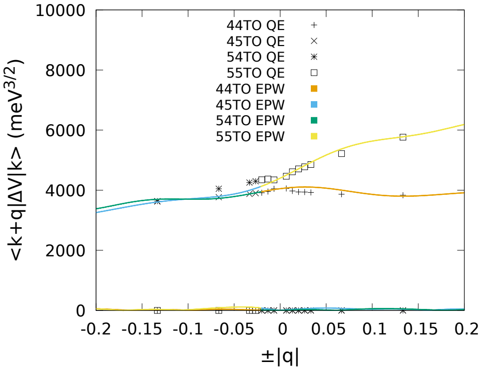


FIG. 8. TO mode, NSCF $48 \times 48 \times 1$ and DFPT $12 \times 12 \times 1$

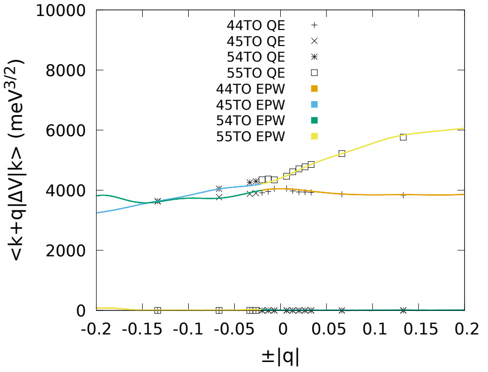


FIG. 9. TO mode, NSCF $24 \times 24 \times 1$ and DFPT $24 \times 24 \times 1$

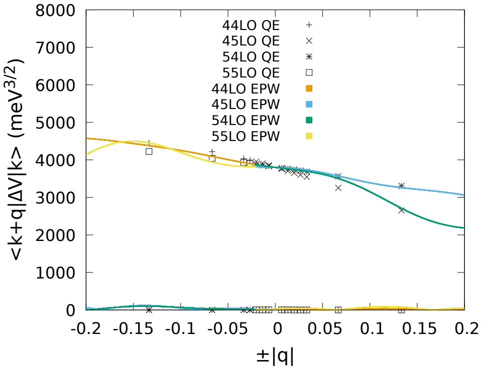


FIG. 10. LO mode, NSCF $24 \times 24 \times 1$ and DFPT $12 \times 12 \times 1$

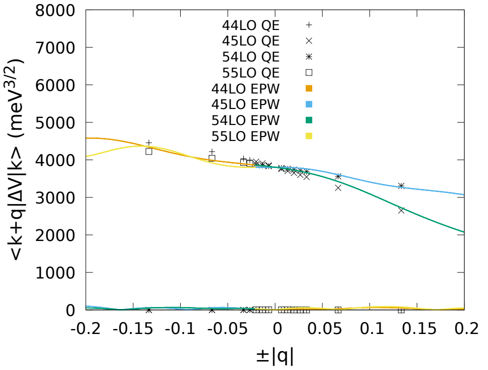


FIG. 11. LO mode, NSCF $48 \times 48 \times 1$ and DFPT $12 \times 12 \times 1$

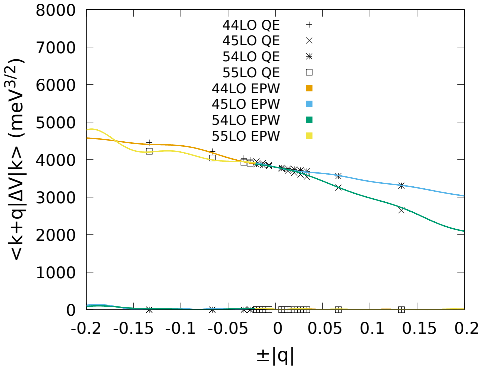


FIG. 12. LO mode, NSCF $24 \times 24 \times 1$ and DFPT $24 \times 24 \times 1$

PANEL 1: Comparison between ab-initio EPC and Wannier-interpolated EPC [$< n = 4, 5; \mathbf{k_1} + \mathbf{q} | \partial_{\mathbf{q}\nu} V | m = 4, 5; \mathbf{k_1} >$]. We compare different NSCF $\mathbf{k}$-point and DFPT $\mathbf{q}$-point grid for different $\nu$ modes, with $\mathbf{q}$ running on the $\Gamma - K$ line and $\mathbf{k_1} = (0.3437500, 0.5953925, 0)$.

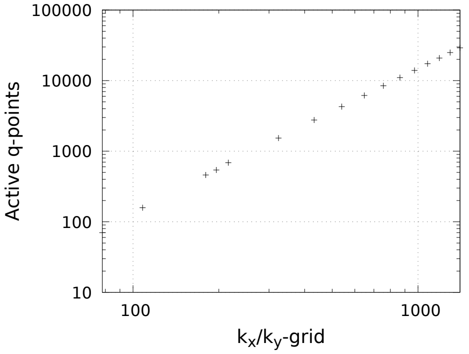


FIG. 13. (a)

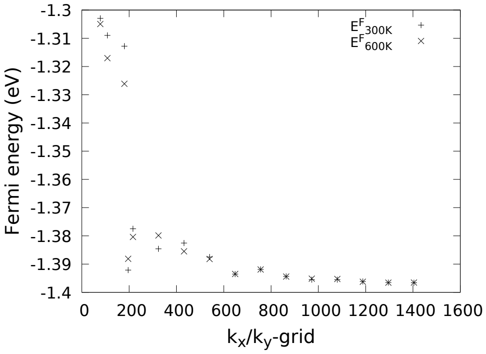


FIG. 14. (b)

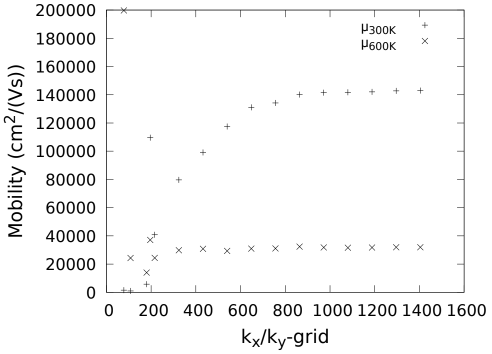


FIG. 15. (c)

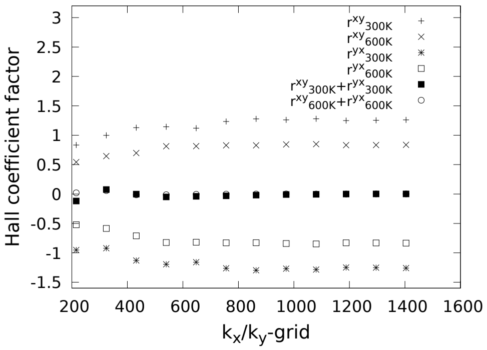


FIG. 16. (d)

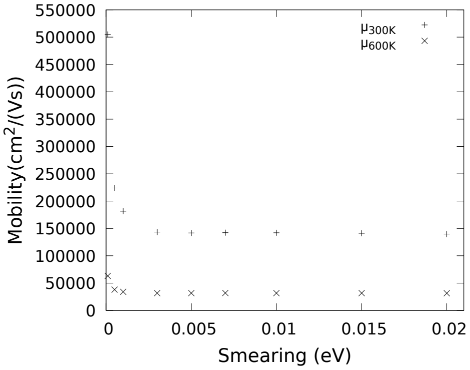


FIG. 17. (e)

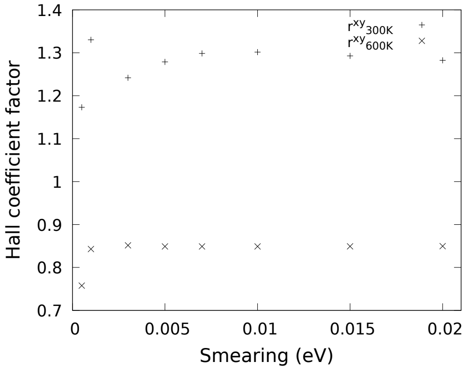


FIG. 18. (f)

PANEL 2: (a) Number of active q-points within the active energy window against the size of the $\mathbf{k}/\mathbf{q}$-point grids. Convergence of (b) Fermi energy, (c) drift mobility and (d) Hall coefficient tensor components against the size of the $\mathbf{k}/\mathbf{q}$-point grids with a fixed smearing of $5meV$. Convergence of (e) drift mobility and (f) Hall coefficient tensor components against the smearing value used at a fixed $1080 \times 1080 \times 1$ $\mathbf{k}/\mathbf{q}$-point grid.

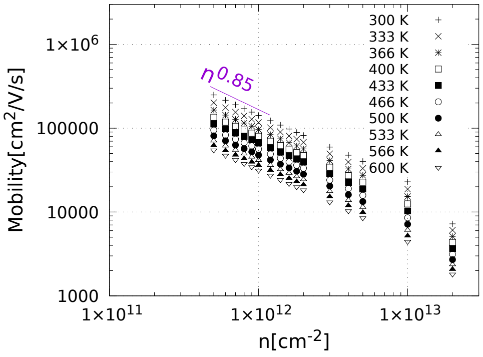


FIG. 19. (a)

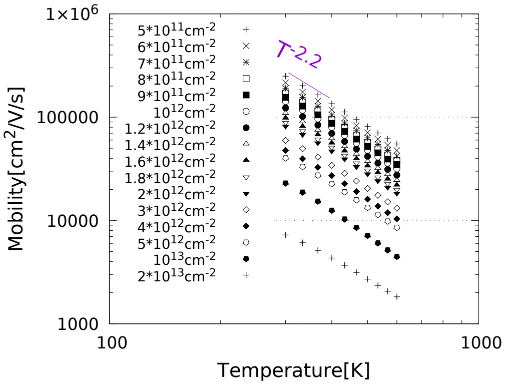


FIG. 20. (b)

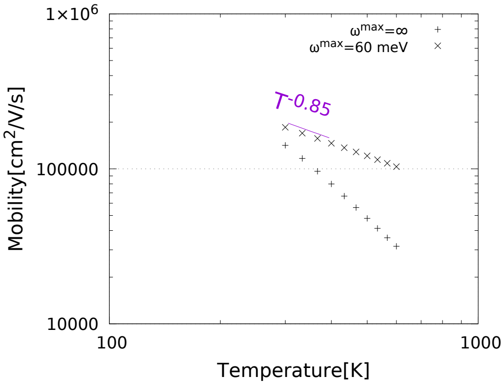


FIG. 21. (c)

PANEL 3: Mobility as a function of (a) carrier concentration and (b) temperature. In (c), we plot the temperature dependence of mobility at a carrier density of $10^{12}cm^{-2}$ when all scattering mechanism are present and when just phonons below $60meV$ are considered.

## VI. DIFFERENCES BETWEEN HOLE AND ELECTRON TRANSPORT COEFFICIENTS

We have seen that the electron-hole symmetry is not fully respected by the electron-phonon coupling matrix elements. Moreover, the electron-hole symmetry is respected by the energy band structure only in the immediate proximity of the Dirac cone center. We show in Panel 5 that, nonetheless, the differences of the transport quantities between holes and electrons are quantitatively very small (for the Hall factor, the sign change is expected because of the sign change of the carriers; the absolute value instead is very similar).

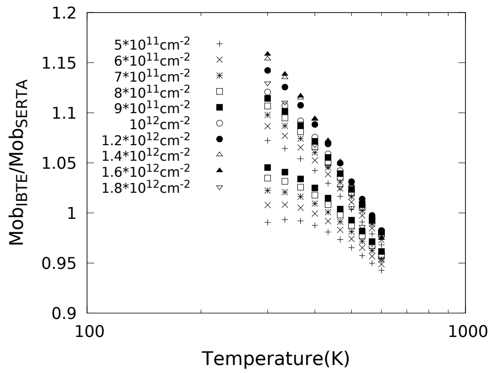


FIG. 22. (a)

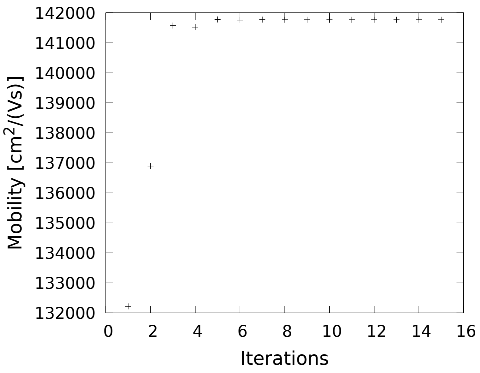


FIG. 23. (b)

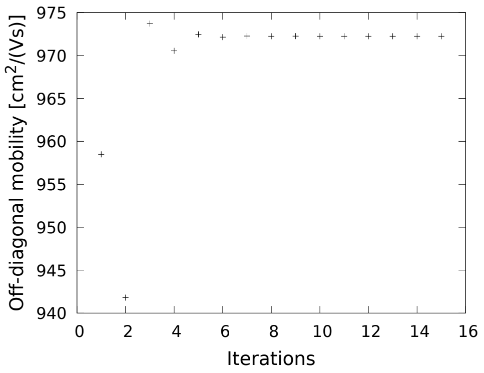


FIG. 24. (c)

PANEL 4: (a) Temperature dependence of the ratio between the solution in the SERTA approximation and the exact solution, for different carrier concentrations; convergence with respect to the iterations of (b) mobility and (c) non-zero out of diagonal component of the mobility tensor when a magnetic field is present; the carrier concentration is $10^{12} cm^{-2}$ and computational parameter as in Tab. I

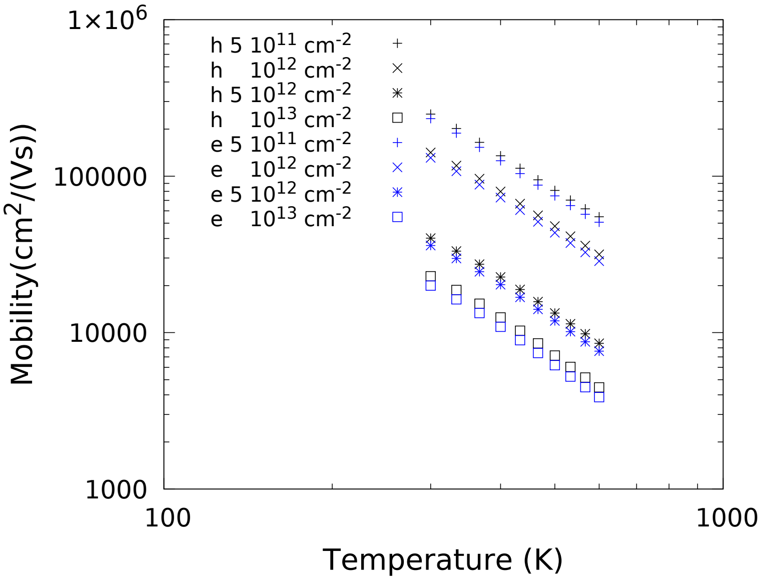


FIG. 25. (a)

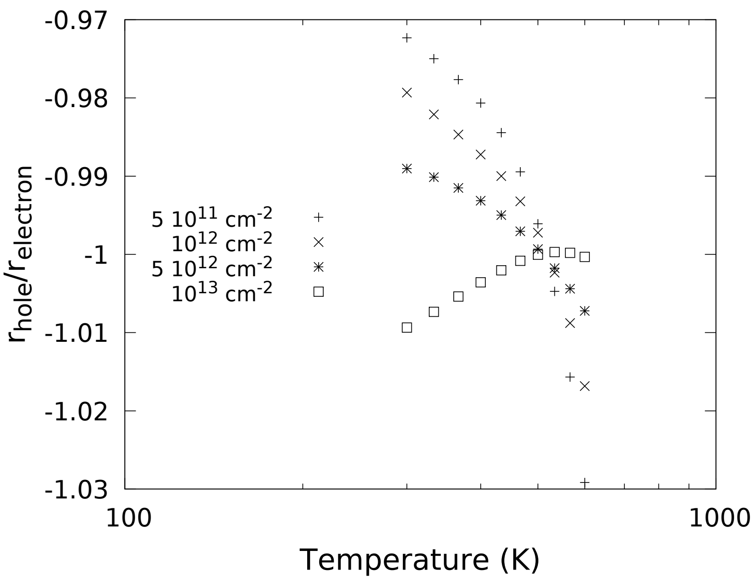


FIG. 26. (b)

PANEL 5: Temperature dependence, for different values of carrier concentration, of (a) hole and electron mobility; (b) ratio of hole and electron Hall coefficient factors.

## VII. INVERSE SCATTERING TIME

The inverse scattering times for different carrier concentration, different phonon cutoffs and grids are given both in the main text and in Panel 6. We mention that the evident asymmetry of the inverse scattering time around the Fermi level is due to the emission of optical phonons, and absence of absorption; we checked that upon increase of temperature (up to 2000K) a more symmetric shape is obtained because optical phonons become populated and absorption is possible.

The comparison between scattering models presented in the main text of this article and ab-initio calculations for the the regime of very low temperatures has been already discussed in the existing literature [29, 30]. For the intermediate regime, we refer to Panel 6; here we show that, upon removal of optical phonon scattering and usage of a "adaptive" smearing scheme (see in the sections above), the inverse scattering time is well described by a linear slope in energy.

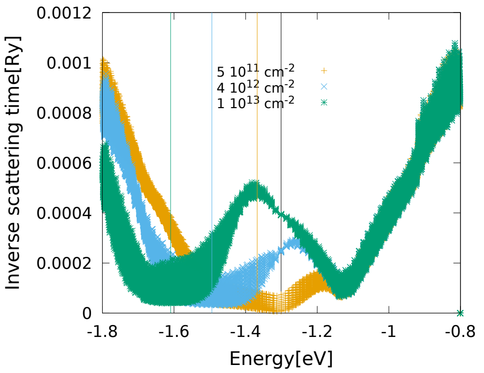


FIG. 27. (a)

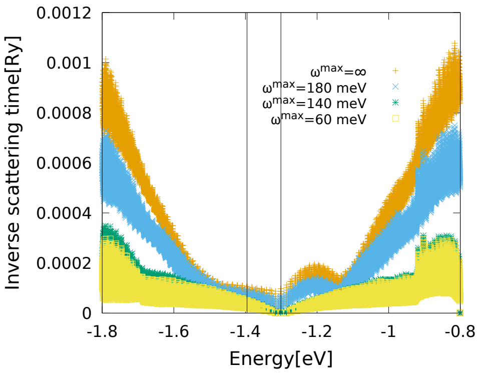


FIG. 28. (b)

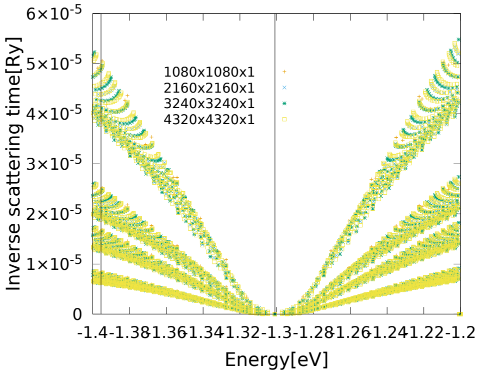


FIG. 29. (c)

PANEL 6: Inverse scattering time as a function of electronic energy for (a) different densities for temperatures going from $300K$ to $600K$ (the vertical lines indicate the center of the Dirac cone [black] and the Fermi levels at various densities [corresponding colours]; since the Fermi level does not change much with temperature, we plot just the 300K one); (b) Inverse scattering times as a function of the phonon cutoff for a density of $10^{-12}cm^{-2}$ and temperatures going from 300 to $600K$ (the Fermi level at $300K$ and the center of the Dirac cone are indicated with vertical lines) ; (c) convergence of inverse scattering time near the Dirac cone with respect to the grid increase for a density of $10^{-12}cm^{-2}$, temperatures $100K, 200K, 300K$ and $600K$ and a phonon cutoff of $60meV$ (the Fermi level at $300K$ and the center of the Dirac cone are indicated with vertical lines)

## VIII. HALL FACTOR MODEL

We can find an analytic formula for the Hall coefficient in the approximation of conic bands, when the magnetic field is without losing generality $\mathbf{B} = B_z\hat{z}$:

$$r = \frac{n_e|e|}{B_z}\frac{\sigma_{12}}{\sigma_{11}^2} \propto -n_e \frac{\sum_n (-1)^n \int_{-\infty}^{\infty} d\epsilon \frac{\partial f_n^0}{\partial \epsilon} \tau_n^{(0),2}(\epsilon)}{\left(\sum_n \int_{-\infty}^{\infty} d\epsilon\epsilon \frac{\partial f_n^0}{\partial \epsilon} \tau_n^{(0)}(\epsilon)\right)^2} \tag{8}$$

where $\epsilon$ is taken with respect to $E_D$, or $\tau_n^{(0)}(\epsilon)$ can be taken from analytical expressions if they are known (see below for more details) or can be defined from the *ab-initio* results as:

$$\tau_n^{(0)}(\epsilon) = (-1)^n \frac{v_F^2}{2\pi\epsilon} \int_{-\infty}^{\infty}\int_{-\infty}^{\infty} dk'^x dk'^y \delta(\epsilon^{FP}(k'^x,k'^y) - \epsilon)\tau_n^{FP}(k'^x,k'^y) = (-1)^n \frac{v_F^2 \Omega_{BZ}}{2\pi\epsilon N_{\mathbf{k}}} \sum_{\mathbf{k}} \delta(\epsilon_{n\mathbf{k}}^{FP} - \epsilon)\tau_{n\mathbf{k}}^{FP}. \tag{9}$$

To derive the above formula for $r$, we start writing the Boltzmann equation in the following form ($e = \hbar = 1$) [4, 5]:

$$-\frac{\partial f_{n\mathbf{k}}^0}{\partial \epsilon_{n\mathbf{k}}} \mathbf{v}_{n\mathbf{k}} \cdot \mathbf{E} + \frac{\partial f_{n\mathbf{k}}^0}{\partial \epsilon_{n\mathbf{k}}} (\mathbf{v}_{n\mathbf{k}} \wedge \mathbf{B}) \cdot \nabla_{\mathbf{k}} \chi_{n\mathbf{k}} = \sum_{m\mathbf{k}'} A_{n\mathbf{k},m\mathbf{k}'} \chi_{m\mathbf{k}'}. \tag{10}$$

where the connection with the notation of the main text of this article is readily seen:

$$\mathbf{k} + \mathbf{q} = \mathbf{k}' \tag{11}$$

$$-\frac{\partial f_{n\mathbf{k}}^0}{\partial \epsilon_{n\mathbf{k}}} \chi_{n\mathbf{k}} = \partial_{E^\beta} f_{n\mathbf{k}} \tag{12}$$

$$\tau_{n\mathbf{k}\to m\mathbf{k+q}}^{-1} = \sum_\nu \frac{2\pi}{\hbar} |g_{mn\nu}(\mathbf{k},\mathbf{q})|^2 \times \left[(n_{\mathbf{q}\nu} + 1 - f_{m\mathbf{k+q}}^0)\delta(\epsilon_{n\mathbf{k}} - \epsilon_{m\mathbf{k+q}} - \hbar\omega_{\mathbf{q}\nu}) + (n_{\mathbf{q}\nu} + f_{m\mathbf{k+q}}^0)\delta(\epsilon_{n\mathbf{k}} - \epsilon_{m\mathbf{k+q}} + \hbar\omega_{\mathbf{q}\nu})\right] =$$

$$= \frac{1 - f_{m\mathbf{k+q}}^0}{1 - f_{n\mathbf{k}}^0} \sum_\nu \frac{2\pi}{\hbar} |g_{mn\nu}(\mathbf{k},\mathbf{q})|^2 \times \left[(n_{\mathbf{q}\nu} + 1)\delta(\epsilon_{n\mathbf{k}} - \epsilon_{m\mathbf{k+q}} - \hbar\omega_{\mathbf{q}\nu}) + n_{\mathbf{q}\nu}\delta(\epsilon_{n\mathbf{k}} - \epsilon_{m\mathbf{k+q}} + \hbar\omega_{\mathbf{q}\nu})\right] \equiv \frac{1 - f_{m\mathbf{k+q}}^0}{1 - f_{n\mathbf{q}}^0} W_{n\mathbf{k}\to m\mathbf{k+q}} \tag{13}$$

$$\tau_{n\mathbf{k}\to m\mathbf{k+q}}^{-1} \partial_{E^\beta} f_{n\mathbf{k}} = \frac{1}{k_B T} f_{n\mathbf{k}}^0 (1 - f_{m\mathbf{k+q}}^0) W_{n\mathbf{k}\to m\mathbf{k+q}} \chi_{n\mathbf{k}} \equiv \frac{1}{k_B T} \Pi_{n\mathbf{k},m\mathbf{k+q}}^0 \chi_{n\mathbf{k}} = \frac{1}{k_B T} \Pi_{m\mathbf{k+q},n\mathbf{k}}^0 \chi_{n\mathbf{k}} \tag{14}$$

$$\tau_{m\mathbf{k+q}\to n\mathbf{k}}^{-1} \partial_{E^\beta} f_{m\mathbf{k+q}} = \frac{1}{k_B T} f_{m\mathbf{k+q}}^0 (1 - f_{n\mathbf{k}}^0) W_{m\mathbf{k+q}\to n\mathbf{k}} \chi_{m\mathbf{k+q}} \equiv \frac{1}{k_B T} \Pi_{m\mathbf{k+q},n\mathbf{k}}^0 \chi_{m\mathbf{k+q}} = \frac{1}{k_B T} \Pi_{n\mathbf{k},m\mathbf{k+q}}^0 \chi_{m\mathbf{k+q}} \tag{15}$$

$$A_{n\mathbf{k},m\mathbf{k+q}} = \frac{1}{k_B T} \left[\Pi_{n\mathbf{k},m\mathbf{k+q}}^0 - \delta_{n\mathbf{k},m\mathbf{k+q}} \sum_{m''\mathbf{k}''} \Pi_{m''\mathbf{k}'',m\mathbf{k+q}}^0\right] \tag{16}$$

where we have used that $(1+n_{\mathbf{q}\nu}-f^0_{m\mathbf{k+q}})f^0_{n\mathbf{k}}(1-f^0_{n\mathbf{k}})\delta(\epsilon_{n\mathbf{k}}-\epsilon_{m\mathbf{k+q}}-\hbar\omega_{\mathbf{q}\nu}) = f^0_{n\mathbf{k}}(1-f^0_{n\mathbf{k+q}})(n_{\mathbf{q}\nu}+1)\delta(\epsilon_{n\mathbf{k}}-\epsilon_{m\mathbf{k+q}}-\hbar\omega_{\mathbf{q}\nu})$, $(n_{\mathbf{q}\nu}+f^0_{m\mathbf{k+q}})f^0_{n\mathbf{k}}(1-f^0_{n\mathbf{k}})\delta(\epsilon_{n\mathbf{k}}-\epsilon_{m\mathbf{k+q}}+\hbar\omega_{\mathbf{q}\nu}) = f^0_{n\mathbf{k}}(1-f^0_{n\mathbf{k+q}})n_{\mathbf{q}\nu}\delta(\epsilon_{n\mathbf{k}}-\epsilon_{m\mathbf{k+q}}+\hbar\omega_{\mathbf{q}\nu})$ and $f^0_{n\mathbf{k}}(1-f^0_{m\mathbf{k+q}})(n_{\mathbf{q}\nu}+1)\delta(\epsilon_{n\mathbf{k}}-\epsilon_{m\mathbf{k+q}}-\hbar\omega_{\mathbf{q}\nu}) = f^0_{m\mathbf{k+q}}(1-f^0_{n\mathbf{k}})n_{\mathbf{q}\nu}\delta(\epsilon_{n\mathbf{k}}-\epsilon_{m\mathbf{k+q}}-\hbar\omega_{\mathbf{q}\nu})$,$f^0_{n\mathbf{k}}(1-f^0_{m\mathbf{k+q}})n_{\mathbf{q}\nu}\delta(\epsilon_{n\mathbf{k}}-\epsilon_{m\mathbf{k+q}}+\hbar\omega_{\mathbf{q}\nu}) = f^0_{m\mathbf{k+q}}(1-f^0_{n\mathbf{k}})(n_{\mathbf{q}\nu}+1)\delta(\epsilon_{n\mathbf{k}}-\epsilon_{m\mathbf{k+q}}+\hbar\omega_{\mathbf{q}\nu})$; notice that these relations hold exactly with the Dirac delta. When we approximate the Dirac delta via Gaussian functions, the previous relations are only approximately true. We check in our calculations though that if we still use the detailed balance relations the error is very small. Indeed we replace:

$$\tau^{-1}_{n\mathbf{k}\to m\mathbf{k+q}} \to \sum_{\nu}\frac{2\pi}{\hbar}|g_{mn\nu}(\mathbf{k},\mathbf{q})|^2\times\left[(n_{\mathbf{q}\nu}+1-f^0_{n\mathbf{k}})\delta(\epsilon_{n\mathbf{k}}-\epsilon_{m\mathbf{k+q}}+\hbar\omega_{\mathbf{q}\nu})+(n_{\mathbf{q}\nu}+f^0_{n\mathbf{k}})\delta(\epsilon_{n\mathbf{k}}-\epsilon_{m\mathbf{k+q}}-\hbar\omega_{\mathbf{q}\nu})\right]\times\frac{f^0_{m\mathbf{k+q}}(1-f^0_{m\mathbf{k+q}})}{f^0_{n\mathbf{k}}(1-f^0_{n\mathbf{k}})}$$

and verify that the final results is not influenced by this substitution.

With the previous relations it can also be shown that the $\tau^{(0),-1}_{n\mathbf{k}}$ as defined in Ref. [2] is related to the diagonal part of $A_{n\mathbf{k},m\mathbf{k+q}}$ by $A_{n\mathbf{k},n\mathbf{k}} = \frac{\partial f^0_{n\mathbf{k}}}{\partial\epsilon_{n\mathbf{k}}}\tau^{(0),-1}_{n\mathbf{k}}$.

If we were able to diagonalize the real symmetric scattering matrix $A_{n\mathbf{k},m\mathbf{k+q}}$ we could rewrite the Boltzmann equation in the diagonal basis $\{\overline{n\mathbf{k}}\}$ such that $D_{\overline{n\mathbf{k}},\overline{m\mathbf{k}'}} = U_{\overline{n\mathbf{k}},l\mathbf{p}}A_{l\mathbf{p},j\mathbf{b}}U^\dagger_{j\mathbf{b},\overline{m\mathbf{k}'}}$, where $U$ is the matrix of basis change between the basis $\{\overline{n\mathbf{k}}\}$ and $\{n\mathbf{k}\}$ and Einstein notation is used. The Boltzmann equation would then be exactly solved at linear order in $\mathbf{B}$ by:

$$\chi_{n\mathbf{k}} = -\left(U^\dagger D^{-1}U\right)_{n\mathbf{k},m\mathbf{k}'}\frac{\partial f^0_{m\mathbf{k}'}}{\partial\epsilon_{m\mathbf{k}'}}\mathbf{v}_{m\mathbf{k}'}\cdot\mathbf{E}-\left(U^\dagger D^{-1}U\right)_{n\mathbf{k},m\mathbf{k}'}\frac{\partial f^0_{m\mathbf{k}'}}{\partial\epsilon_{m\mathbf{k}'}}\left(\mathbf{v}_{m\mathbf{k}'}\wedge\mathbf{B}\right)\cdot\left[\nabla_{\mathbf{k}'}\left\{\left(U^\dagger D^{-1}U\right)_{m\mathbf{k}',l\mathbf{p}}\frac{\partial f^0_{l\mathbf{p}}}{\partial\epsilon_{l\mathbf{p}}}\mathbf{v}_{l\mathbf{p}}\cdot\mathbf{E}\right\}\right]. \tag{17}$$

The above equation is equivalent to exactly solve the Boltzmann equation as explained in section I. We can simplify the above expression in order to try to describe some physical properties without having to do all the numerics, by setting $\left(U^\dagger D^{-1}U\right)_{n\mathbf{k},m\mathbf{k}'} = 1/\left(\frac{\partial f^0_{n\mathbf{k}}}{\partial\epsilon_{n\mathbf{k}}}\right)\delta_{n\mathbf{k},m\mathbf{k}'}\tau^{(0)}_{n\mathbf{k}}$. In this case the Boltzmann equation becomes:

$$-\mathbf{v}_{n\mathbf{k}}\cdot\mathbf{E}+(\mathbf{v}_{n\mathbf{k}}\wedge\mathbf{B})\cdot\nabla_{\mathbf{k}}\chi_{n\mathbf{k}} = \tau^{(0),-1}_{n\mathbf{k}}\chi_{n\mathbf{k}} \tag{18}$$

and to first order in the $\mathbf{B}$ field this equation is solved by:

$$\chi_{n\mathbf{k}} = -\mathbf{v}_{n\mathbf{k}}\cdot\mathbf{E}\tau^{(0)}_{n\mathbf{k}}-(\mathbf{v}_{n\mathbf{k}}\wedge\mathbf{B})\cdot\left[\nabla_{\mathbf{k}}\left(\mathbf{v}_{n\mathbf{k}}\cdot\mathbf{E}\tau^{(0)}_{n\mathbf{k}}\right)\right]\tau^{(0)}_{n\mathbf{k}} \tag{19}$$

The above expression may be obtained in the Self Energy Time Approximation (SERTA). Of course, the validity of the above expression is extendend beyond the SERTA approximation if we are able to obtain an expression for the out of equilibrium population which is of the same form. If, by any other procedure or approximation, we can substitute the collisional integral of the r.h.s. member of the Boltzmann equation with a simple expression containing just a function of $\tau^{(0)}_{n\mathbf{k}}$, then the derivation is still valid. This is done for example in Refs. [21, 31], with an *exact* procedure once that it is assumed that the energy bands are conic and that the scattering mechanism are quasielastic (valid for low temperatures and low doping). In this case the above expression for the out of equilibrium population is exact and also the derivation of the model for the Hall factor that follows below is to be intended as exact. If we consider also inelastic scatterings (optical phonons), then Eq. 33 is to be intended as an approximation.

To eliminate the electric field, we notice that even with the magnetic field each term in the Boltzmann equation is coherently linear in the electric field, so that the equation must be satisfied for every possible value and orientation of the electric field. Therefore we define $\chi_{n\mathbf{k}} = \mathbf{\Phi}_{n\mathbf{k}}\cdot\mathbf{E}$ and we must have, for each vectorial component:

$$\mathbf{\Phi}_{n\mathbf{k}} = -\mathbf{v}_{n\mathbf{k}}\tau^{(0)}_{n\mathbf{k}}-(\mathbf{v}_{n\mathbf{k}}\wedge\mathbf{B})\cdot\nabla_{\mathbf{k}}\left(\mathbf{v}_{n\mathbf{k}}\tau^{(0)}_{n\mathbf{k}}\right)\tau^{(0)}_{n\mathbf{k}} \tag{20}$$

In 2D for graphene, it is convenient to rewrite these vectorial equations in cylindrical components $[(k^\rho,k^\theta)\equiv(\rho,\theta)]$ around the special point $K$:

$$\Phi^\rho_{n\mathbf{k}}\hat{\rho}+\Phi^\theta_{n\mathbf{k}}\hat{\theta} = -\left(v^\rho_{n\mathbf{k}}\hat{\rho}+v^\theta_{n\mathbf{k}}\hat{\theta}\right)\tau^{(0)}_{n\mathbf{k}}-\sum_{LMN}\epsilon_{LMN}v^L_{n\mathbf{k}}B^M\nabla^N_{\mathbf{k}}\left[(v^\rho_{n\mathbf{k}}\hat{\rho}+v^\theta_{n\mathbf{k}}\hat{\theta})\tau^{(0)}_{n\mathbf{k}}\right]\tau^{(0)}_{n\mathbf{k}} \tag{21}$$

where the components of the vectors inside the vector product are intended to be cylindrical and all the vectors are considered to be functions of $(\rho,\theta)$, and $\epsilon_{LMN}$ is the Levi-Civita tensor. Our approximation consist in taking $\epsilon_{n\mathbf{k}} = \epsilon_n(\rho) = (-1)^n v_F\rho$ where we reduce the problem to only the $\pi$ $(n=0)$ and $\pi^*$ $(n=1)$ bands, $v_F$ is the modulus of the Fermi velocity, so that the band velocity is only radial. In this way also $\tau^{(0)}_{n\mathbf{k}}$ is only function of $\rho$ because the scattering time has the same symmetries of the energy states [4] (of course this approximation holds only in the immediate proximity of $E_D$). Moreover we are interested in the case of a magnetic field along the z-direction. It follows that the only term which is retained is the one with $L=1, M=3, N=2$:

$$\Phi^\rho_{n\mathbf{k}}\hat{\rho}+\Phi^\theta_{n\mathbf{k}}\hat{\theta} = -\left((-1)^n v_F\hat{\rho}\right)\tau^{(0)}_{n\mathbf{k}}+v_F B^z\nabla^\theta_{\mathbf{k}}\left(v_F\hat{\rho}\tau^{(0)}_{n\mathbf{k}}\right)\tau^{(0)}_{n\mathbf{k}} \tag{22}$$

which becomes:

$$\Phi^\rho_{n\mathbf{k}}\hat{\rho}+\Phi^\theta_{n\mathbf{k}}\hat{\theta} = -\left((-1)^n v_F\hat{\rho}\right)\tau^{(0)}_{n\mathbf{k}}+v_F B^z\frac{1}{\rho}\frac{\partial}{\partial\theta}\left(v_F\hat{\rho}\tau^{(0)}_{n\mathbf{k}}\right)\tau^{(0)}_{n\mathbf{k}} \tag{23}$$

Using the fact that $\frac{\partial}{\partial\theta}\hat{\rho} = \hat{\theta}$ we obtain to first order in the $\mathbf{B}$ field:

$$\Phi^{\rho}_{n\mathbf{k}} = -(-1)^n v_F \tau^{(0)}_{n\mathbf{k}} \tag{24}$$

$$\Phi^{\theta}_{n\mathbf{k}} = v_F^2 B^z \frac{1}{\rho}\tau^{(0),2}_{n\mathbf{k}} \tag{25}$$

Now we define the quantity $S^{pol.}_{ij} = v_i \Phi_j$ (dropping for the moment $\{n\mathbf{k}\}$), which, when integrated, gives the conductivity. We transform these quantities in the cartesian components by:

$$S^{cart.}_{ij} = \sum_{k,l} U^{\dagger}_{ik} S^{pol.}_{kl} U_{lj} \tag{26}$$

where the $S$ on the left is expressed in cartesian indexes, while on the right in polar. The matrix $U$ is the matrix of basis change:

$$U = \begin{pmatrix} \cos(\theta) & \sin(\theta) \\ -\sin(\theta) & \cos(\theta) \end{pmatrix} \tag{27}$$

and therefore obtain:

$$S^{cart.} = v^{\rho} \begin{pmatrix} \Phi^{\rho}\cos^2(\theta) - \Phi^{\theta}\sin(\theta)\cos(\theta) & \Phi^{\rho}\cos(\theta)\sin(\theta) + \Phi^{\theta}\cos^2(\theta) \\ \Phi^{\rho}\sin(\theta)\cos(\theta) - \Phi^{\theta}\sin^2(\theta) & \Phi^{\rho}\sin^2(\theta) + \Phi^{\theta}\sin(\theta)\cos(\theta) \end{pmatrix} \tag{28}$$

We now express the conductivity tensor:

$$\sigma^{cart.} = -\frac{2}{\Omega\Omega_{BZ}} \sum_n \int_0^{\infty}\int_0^{2\pi} \rho d\rho d\theta v^{\rho}_n \frac{\partial f^0_n}{\partial\epsilon}(\epsilon_n(\rho)) \begin{pmatrix} \Phi^{\rho}_n\cos^2(\theta) - \Phi^{\theta}_n\sin(\theta)\cos(\theta) & \Phi^{\rho}_n\cos(\theta)\sin(\theta) + \Phi^{\theta}_n\cos^2(\theta) \\ \Phi^{\rho}_n\sin(\theta)\cos(\theta) - \Phi^{\theta}_n\sin^2(\theta) & \Phi^{\rho}_n\sin^2(\theta) + \Phi^{\theta}_n\sin(\theta)\cos(\theta) \end{pmatrix} \tag{29}$$

Integrating in the angular dependence (and remembering that $\Phi^{r,\phi}$ and $\frac{\partial f^0_n}{\partial\epsilon}$ do not have angular dependence, and putting $v^{\rho}_n \sim (-1)^n v^F$) we have:

$$\sigma^{cart.} = -(2\pi)^{-1} v^F \sum_n (-1)^n \int_0^{\infty} \rho d\rho \frac{\partial f^0_n}{\partial\epsilon}(\epsilon_n(\rho)) \begin{pmatrix} \Phi^{\rho}_n & \Phi^{\theta}_n \\ -\Phi^{\theta}_n & \Phi^{\rho}_n \end{pmatrix} \tag{30}$$

where we notice that in absence of a magnetic field, the tensor would be diagonal as expected for symmetry reasons, while in presence of a magnetic field the off diagonal components are different in sign. We now insert the values for $\Phi^r$ and $\Phi^{\theta}$ and find :

$$\sigma_{xx} = (2\pi)^{-1} v^{F,2} \sum_n \int_0^{\infty} \rho d\rho \frac{\partial f^0_n}{\partial\epsilon}(\epsilon_n(\rho)) \tau^{(0)}_n(\epsilon_n(\rho)) \tag{31}$$

$$\sigma_{xy} = -(2\pi)^{-1} v^{F,3} B_z \sum_n (-1)^n \int_0^{\infty} \rho d\rho \frac{\partial f^0_n}{\partial\epsilon}(\epsilon_n(\rho)) \frac{1}{\rho}\tau^{(0),2}_n(\epsilon_n(\rho)) \tag{32}$$

where we have dropped the $\mathbf{k}$ index from the scattering time because it depends just on the radial coordinate. It follows, using $\epsilon_n(\rho) = (-1)^n v^F \rho$ (restoring the $\hbar$):

$$r = \frac{n_e|e|}{B_z}\frac{\sigma_{12}}{\sigma^2_{11}} = -2\pi v^{F,2}\hbar^2 n_e \frac{\sum_n (-1)^n \int_{-\infty}^{\infty} d\epsilon \frac{\partial f^0_n}{\partial\epsilon}\tau^{(0),2}_n(\epsilon)}{\left(\sum_n (-1)^n \int_{-\infty}^{\infty} d\epsilon\epsilon \frac{\partial f^0_n}{\partial\epsilon}\tau^{(0)}_n(\epsilon)\right)^2} \tag{33}$$

where all the quantities under integration sign are to be intended as functions of the integration variable $\epsilon$ only. The $(-1)^n$ in the denominator compensate the negative sign coming from the area element for $\epsilon < 0$, so that the contributions to the diagonal components are always positive. On the contrary the $(-1)^n$ in the numerator subtract the contributions between hole and electron transport; in condition of perfect hole-electron simmetry of the band structure (low temperatures and no doping) the two contributions tends to cancel out and $r$ becomes very small. If the Fermi level is moved slightly from $E_D$, then one band contribution will dominate and we will obtain a non zero $r$; since the hole and electron mobility in graphene is practically the same, especially at very low doping (see previous sections), the value of $r$ is expected to be anti-symmetric around the Dirac cone (as it results from ab-initio calculations, see previous section).

Now, we will use the above formulas by inputting the first principles evaluation of $\tau^{(0)}_{n\mathbf{k}} = \tau^{(0)}_n(k^{\rho}(\epsilon))$. For the relaxation time, we define (the superscript FP means First Principle):

$$\tau^{(0)}(k^{\rho}(\epsilon)) = \frac{1}{2\pi}\int_0^{2\pi} dk'^{\theta}\tau^{(0),FP}_n(k^{\rho}(\epsilon), k'^{\theta}) = \frac{1}{2\pi k^{\rho}(\epsilon)}\int_0^{\infty}\int_0^{2\pi} dk'^{\rho}k'^{\rho}\delta(k'^{\rho} - k^{\rho}(\epsilon))dk'^{\theta}\tau^{(0),FP}_n(k'^{\rho}, k'^{\theta}) = \tag{34}$$

$$\frac{1}{2\pi k^{\rho}(\epsilon)}\int_0^{\infty}\int_0^{2\pi} dk'^{\rho}k'^{\rho}\delta(\frac{\epsilon'(k'^{\rho})}{v_F} - k^{\rho}(\epsilon))dk'^{\theta}\tau^{(0),FP}_n(k'^{\rho}, k'^{\theta}) = \frac{1}{2\pi k^{\rho}(\epsilon)}\int_{-\infty}^{\infty}\int_{-\infty}^{\infty} dk'^x dk'^y \delta(\frac{\epsilon'(k'^x, k'^y)}{v_F} - k^{\rho}(\epsilon))\tau^{(0),FP}_n(k'^x, k'^y) \tag{35}$$

where $\epsilon'(k^x, k^y)$ is the linear expression of the energy as a function of $\mathbf{k}$. Now, as long as we know $\tau$ for energies which are given by the ab-initio calculations, we substitute the true energies in the expression above to obtain:

$$\tau^{(0)}(k^\rho(\epsilon)) = \frac{1}{2\pi k^\rho(\epsilon)} \int_{-\infty}^{\infty}\int_{-\infty}^{\infty} dk'^x dk'^y \delta(\frac{\epsilon^{FP}(k'^x, k'^y)}{v_F} - k^\rho(\epsilon))\tau_n^{(0),FP}(k'^x, k'^y) \tag{36}$$

and bringing eveything in energy (and restoring $\hbar$):

$$\tau_n^{(0)}(\epsilon) = (-1)^n \frac{v_F^2}{2\pi\epsilon} \int_{-\infty}^{\infty}\int_{-\infty}^{\infty} dk'^x dk'^y \delta(\epsilon^{FP}(k'x, k'y) - \epsilon)\tau_n^{(0),FP}(k'^x, k'^y) = (-1)^n \frac{v_F^2 \Omega_{BZ}\hbar^2}{2\pi\epsilon N_{\mathbf{k}}} \sum_{\mathbf{k}} \delta(\epsilon_{n\mathbf{k}}^{FP} - \epsilon)\tau_{n\mathbf{k}}^{(0),FP} \tag{37}$$

where we note that the minus sign is compensated by the fact that $\epsilon < 0$ for $n = 1$. In using the above equation in general we have to introduce a cutoff to avoid that $\tau^{(0)}(\epsilon)$ numerically scales as $\frac{1}{\epsilon}$ near 0, even if the scattering time tends to a finite value in that region. The reason is that, for any given grid of $\mathbf{k}$ points, there exist a zone near the Dirac cone where the density of states is not sufficiently well represented.

We now discuss, in a more extended way with respect to the main text of the article, the expected behaviour of the Hall factor by evaluation of Eq. 33 in different temperature and doping regimes. We drop the (0) apex for the scattering time for notation easiness. We mainly identify four regimes where $r$ has distinct behaviours:

1. Bloch-Gruneisen regime ($0 < T \ll T_{B.-G.}$ where $T_{B.-G.} = 2\hbar v_{TA/LA} k_F/k_B$). In this regime obtaining a close expression of $\tau_n$ as a function of energy alone is non-trivial [21, 25, 32], but it can be evaluated around the Fermi Level as $\tau(E_F) \propto \frac{(k_BT)^4}{E_F}$. Moreover, all the quantities in Eq. 33 at low temperatures may be evaluated at $\epsilon = E_F$. With this approximation we have that the Hall factor scales as $r \propto n/D(E_F)^2 \propto 1$ (where $D(E_F)$ is the density of states at the Fermi level and the number of carriers at low temperatures is proportional to $\pm \int_{E_F}^{E_D=0} E dE = \pm E_F^2/2$) and so it is fairly independent of temperature and doping.

2. Equipartition regime at low doping($T_{B.-G.} \ll T < 270K$ and $n < 10^{13} cm^{-2}$) where the optical phonons are not yet an important scattering mechanism and we have just $TA/LA$ lattice vibrations. In this regime, where $\hbar\omega_{\mathbf{q},TA/LA} << k_BT$ the expression for the scattering time is found to be $\tau^{-1}(\epsilon_{n\mathbf{k}}) \propto |\epsilon_{n\mathbf{k}}| k_BT$. In the approximation of linear band dispersion around the Fermi Dirac level, we have $\tau_n^{-1}(\epsilon) \propto |\epsilon| k_BT$. This expression is obtained from Eq. 2 just by considering scatterings between electrons as quasielastic (given that the acoustic phonon scale is very small if compared to the bands energies scale), that the electronic population do not change appreciably over a length of $\hbar\omega_{\mathbf{q},TA/LA}$ around the Fermi level and that the phonon population can be expressed as $N_{\mathbf{q},TA/LA} = \frac{k_BT}{\hbar\omega_{\mathbf{q},TA/LA}}$. These assumptions all hold true in this regime. The seemingly conclusion is that the integral at the numerator of Eq. 33 is always divergent but for $T = 0$, when the derivative of the Fermi-Dirac is actually a Dirac delta and evaluates the numerator as $\tau^2(E_F)$. This result is unphysical, the reason being that Eq. 2 holds true when the many-body spectral function is well approximated by a Lorentzian with vanishing but non zero widths $\Gamma_{n\mathbf{k}}$ (i.e. much smaller than the particle energy as measured from the Fermi level) given by $\tau_{n\mathbf{k}}^{-1} = \frac{2\pi}{\hbar}\Gamma_{n\mathbf{k}}$. Indeed, this is to be treated carefully around the Dirac cone where both the energy and the linewidth goes to 0, and a correction to the linear scaling of $\tau^{-1}$ is expected.

   Moreover, the scattering time of the optical phonons itself is not completely 0, but it is expected to be at $\epsilon = 0$ for the lowest optical mode $A_1'$ at $\mathbf{q} = \mathbf{K}$ [21]:

$$\frac{1}{\tau_{A_1'}(\epsilon = 0)} = \frac{\beta_{\mathbf{K}}^2}{\mu_S} \frac{1}{(\hbar v_F)^2} \frac{\hbar/2}{1 - f^0(0)} \times \left[3N_{A_1'}(1 - f^0(\hbar\omega_{A_1'})) + (N_{A_1'} + 1)(1 - f^0(-\hbar\omega_{A_1'}))\right] \tag{38}$$

   where $\beta_{\mathbf{K}}$ is the optical gauge field, $\omega_{A_1'}$ is the frequency and $N_{A_1'}$ the occupation of the $A_1'$ mode and $\mu_S$ is the graphene mass density. In this case, the inverse scattering time depends both on the temperature and on the position of the Fermi level; since by the way below room temperature $N_{A_1'} < 0.004 \ll 1$ we can simplify the previous expression in:

$$\frac{1}{\tau_{A_1'}(\epsilon = 0)} = \frac{\beta_{\mathbf{K}}^2}{\mu_S} \frac{1}{(\hbar v_F)^2} \frac{\hbar/2}{1 - f^0(0)} \left[3N_{A_1'}(1 - f^0(\hbar\omega_{A_1'})) + (1 - f^0(-\hbar\omega_{A_1'}))\right]. \tag{39}$$

   If we now take $|E_F| << \omega_{A_1'}$, which is true in the low doping regime ($n << 10^{13} cm^{-2}$), we have that the expression can be simplified as:

$$\frac{1}{\tau_{A_1'}(\epsilon = 0)} = \frac{\beta_{\mathbf{K}}^2}{\mu_S} \frac{1}{(\hbar v_F)^2} \hbar \left[3N_{A_1'} \frac{e^{\hbar\omega_{A_1'}/k_BT}}{e^{\hbar\omega_{A_1'}/k_BT} + 1} + \frac{e^{-\hbar\omega_{A_1'}/k_BT}}{e^{-\hbar\omega_{A_1'}/k_BT} + 1}\right] \tag{40}$$

   which evalutes to $\frac{1}{\tau} \approx 7 \times 10^{10} s^{-1}$ at room temperature.

   Also, graphene flakes have finite size and therefore the size of the samples puts a cutoff for the minimum $\mathbf{k}$ vector (and consequently energy states) available in the system. In particular, if we consider a graphene flake of dimensions $1\mu m^2$, then we expect that we cannot get nearer than approximatively 1 meV to the Dirac cone. Of course, for graphene flakes of larger dimensions we can implement smaller cutoffs and expect slightly larger peak values for $r$.

   That said, the temperature and carrier concentration behaviour of the Hall factor in this regime is non-trivial because, as the denominator of Eq. 33 is pretty insensitive to the form of the scattering time around the Dirac cone, we have seen that the

numerator instead it is highly sensitive. Therefore, we expect that if $\frac{E_F-E_d}{k_BT} \gg 1$ the Hall factor is fairly temperature and doping independent, because $\frac{\partial f^0_{n\mathbf{k}}}{\partial \epsilon_{n\mathbf{k}}}$ cuts off the integral near the Dirac cone, whereas if $\frac{E_F-E_d}{k_BT} \ll 1$ we expect a strong doping and temperature dependence for $r$ because the numerator can attain large values while the denominator doesn't change much. In order to evaluate the behaviour of $r$, we implement Eq. 33 with $\tau(\epsilon) \propto \epsilon^{-1}$ (see main text) except for a small region around $\epsilon = 0$, which we cut off from the integration for simplicity. Even though for temperatures above $270K$ the form of the $\tau$ is different from $\frac{1}{\epsilon}$, we can think at this result as the Hall in absence of optical phonons. We decided to use a value of $1meV$ as a cutoff for our calculations.

3. High-temperature regime ($T > 280K$) at low doping: here $E_F$ is near the Dirac cone and the Fermi-Dirac distrubution is not sharp, therefore both hole and electrons contribute to the numerator of Eq. 33 with opposite sign. Here $r$ is expected to be small.

4. High doping regime: in this regime we are far away from the Dirac cone and the model for the Hall factor of Eq. 33 starts to be imprecise quantitatively, and the scattering times have a non-trivial behaviour. Nonetheless, we expect the dependence of $r$ on density of carriers and temperature to be mild.

[1] Samuel Poncé, Elena R. Margine, and Feliciano Giustino. Towards predictive many-body calculations of phonon-limited carrier mobilities in semiconductors. *Phys. Rev. B*, 97:121201, Mar 2018.

[2] Samuel Poncé, Wenbin Li, Sven Reichardt, and Feliciano Giustino. First-principles calculations of charge carrier mobility and conductivity in bulk semiconductors and two-dimensional materials. *Reports on Progress in Physics*, 83(3):036501, feb 2020.

[3] Feliciano Giustino. Electron-phonon interactions from first principles. *Rev. Mod. Phys.*, 89:015003, Feb 2017.

[4] Francesco Macheda and Nicola Bonini. Magnetotransport phenomena in $p$-doped diamond from first principles. *Phys. Rev. B*, 98:201201, Nov 2018.

[5] Mattia Fiorentini and Nicola Bonini. Thermoelectric coefficients of $n$-doped silicon from first principles via the solution of the boltzmann transport equation. *Phys. Rev. B*, 94:085204, Aug 2016.

[6] Feliciano Giustino, Marvin L. Cohen, and Steven G. Louie. Electron-phonon interaction using wannier functions. *Phys. Rev. B*, 76:165108, Oct 2007.

[7] Jonathan R. Yates, Xinjie Wang, David Vanderbilt, and Ivo Souza. Spectral and fermi surface properties from wannier interpolation. *Phys. Rev. B*, 75:195121, May 2007.

[8] Robert F. Snider. Quantum-mechanical modified boltzmann equation for degenerate internal states. *The Journal of Chemical Physics*, 32(4):1051–1060, 1960.

[9] W. Kohn and L. J. Sham. Self-consistent equations including exchange and correlation effects. *Phys. Rev.*, 140:A1133–A1138, Nov 1965.

[10] Stefano Baroni, Stefano de Gironcoli, Andrea Dal Corso, and Paolo Giannozzi. Phonons and related crystal properties from density-functional perturbation theory. *Rev. Mod. Phys.*, 73:515–562, Jul 2001.

[11] Nicola Marzari, Arash A. Mostofi, Jonathan R. Yates, Ivo Souza, and David Vanderbilt. Maximally localized wannier functions: Theory and applications. *Rev. Mod. Phys.*, 84:1419–1475, Oct 2012.

[12] Paolo Giannozzi, Stefano Baroni, Nicola Bonini, Matteo Calandra, Roberto Car, Carlo Cavazzoni, Davide Ceresoli, Guido L Chiarotti, Matteo Cococcioni, Ismaila Dabo, Andrea Dal Corso, Stefano de Gironcoli, Stefano Fabris, Guido Fratesi, Ralph Gebauer, Uwe Gerstmann, Christos Gougoussis, Anton Kokalj, Michele Lazzeri, Layla Martin-Samos, Nicola Marzari, Francesco Mauri, Riccardo Mazzarello, Stefano Paolini, Alfredo Pasquarello, Lorenzo Paulatto, Carlo Sbraccia, Sandro Scandolo, Gabriele Sclauzero, Ari P Seitsonen, Alexander Smogunov, Paolo Umari, and Renata M Wentzcovitch. Quantum espresso: a modular and open-source software project for quantum simulations of materials. *Journal of Physics: Condensed Matter*, 21(39):395502, 2009.

[13] Jesse Noffsinger, Feliciano Giustino, Brad D. Malone, Cheol-Hwan Park, Steven G. Louie, and Marvin L. Cohen. Epw: A program for calculating the electron–phonon coupling using maximally localized wannier functions. *Computer Physics Communications*, 181(12):2140 – 2148, 2010.

[14] S. Poncé, E.R. Margine, C. Verdi, and F. Giustino. Epw: Electron–phonon coupling, transport and superconducting properties using maximally localized wannier functions. *Computer Physics Communications*, 209:116 – 133, 2016.

[15] John P. Perdew and Yue Wang. Accurate and simple analytic representation of the electron-gas correlation energy. *Phys. Rev. B*, 45:13244–13249, Jun 1992.

[16] J. P. Perdew and Alex Zunger. Self-interaction correction to density-functional approximations for many-electron systems. *Phys. Rev. B*, 23:5048–5079, May 1981.

[17] Thibault Sohier, Matteo Calandra, and Francesco Mauri. Density functional perturbation theory for gated two-dimensional heterostructures: Theoretical developments and application to flexural phonons in graphene. *Phys. Rev. B*, 96:075448, Aug 2017.

[18] J. L. Mañes. Symmetry-based approach to electron-phonon interactions in graphene. *Phys. Rev. B*, 76:045430, Jul 2007.

[19] G. Grosso and G.P. Parravicini. *Solid State Physics*. Elsevier Science, 2000.

[20] Cheol-Hwan Park, Nicola Bonini, Thibault Sohier, Georgy Samsonidze, Boris Kozinsky, Matteo Calandra, Francesco Mauri, and Nicola Marzari. Electron–phonon interactions and the intrinsic electrical resistivity of graphene. *Nano Letters*, 14(3):1113–1119, 2014. PMID: 24524418.

[21] Thibault Sohier, Matteo Calandra, Cheol-Hwan Park, Nicola Bonini, Nicola Marzari, and Francesco Mauri. Phonon-limited resistivity of graphene by first-principles calculations: Electron-phonon interactions, strain-induced gauge field, and boltzmann equation. *Phys. Rev. B*, 90:125414, Sep 2014.

[22] S. V. Morozov, K. S. Novoselov, M. I. Katsnelson, F. Schedin, D. C. Elias, J. A. Jaszczak, and A. K. Geim. Giant intrinsic carrier mobilities in graphene and its bilayer. *Phys. Rev. Lett.*, 100:016602, Jan 2008.

[23] K.I. Bolotin, K.J. Sikes, Z. Jiang, M. Klima, G. Fudenberg, J. Hone, P. Kim, and H.L. Stormer. Ultrahigh electron mobility in suspended graphene. *Solid State Communications*, 146(9):351 – 355, 2008.

[24] K. S. Novoselov, V. I. Fal'ko, L. Colombo, P. R. Gellert, M. G. Schwab, and K. Kim. A roadmap for graphene. *Nature*, 490(7419):192–200, 2012.

[25] E. H. Hwang and S. Das Sarma. Acoustic phonon scattering limited carrier mobility in two-dimensional extrinsic graphene. *Phys. Rev. B*, 77:115449, Mar 2008.

[26] K. M. Borysenko, J. T. Mullen, E. A. Barry, S. Paul, Y. G. Semenov, J. M. Zavada, M. Buongiorno Nardelli, and K. W. Kim. First-principles analysis of electron-phonon interactions in graphene. *Phys. Rev. B*, 81:121412, Mar 2010.

[27] Tue Gunst, Troels Markussen, Kurt Stokbro, and Mads Brandbyge. First-principles method for electron-phonon coupling and electron mobility: Applications to two-dimensional materials. *Phys. Rev. B*, 93:035414, Jan 2016.

[28] Oscar D Restrepo, Kevin E Krymowski, Joshua Goldberger, and Wolfgang Windl. A first principles method to simulate electron mobilities in 2d materials. *New Journal of Physics*, 16(10):105009, oct 2014.

[29] Cheol-Hwan Park, Feliciano Giustino, Marvin L. Cohen, and Steven G. Louie. Velocity renormalization and carrier lifetime in graphene from the electron-phonon interaction. *Phys. Rev. Lett.*, 99:086804, Aug 2007.

[30] Matteo Calandra and Francesco Mauri. Electron-phonon coupling and electron self-energy in electron-doped graphene: Calculation of angular-resolved photoemission spectra. *Phys. Rev. B*, 76:205411, Nov 2007.

[31] T. Kawamura and S. Das Sarma. Phonon-scattering-limited electron mobilities in $\mathrm{al}_x\mathrm{ga}_{1-x}\mathrm{as}$/gaas heterojunctions. *Phys. Rev. B*, 45:3612–3627, Feb 1992.

[32] Khoe Van Nguyen and Yia-Chung Chang. Full consideration of acoustic phonon scatterings in two-dimensional dirac materials. *Phys. Chem. Chem. Phys.*, 22:3999–4009, 2020.
